# Supplementary material for: Exact SU(2) Yang-Mills Waves from a Simple Ansatz
Source: arXiv:2605.04964 source file (2026-11-15)
Supplement: Supplementary file 1 [file sm-EYMW-v1A-arxiv.tex]

\documentclass[aps,pra,reprint,aps,onecolumn,superscriptaddress]{revtex4}

\usepackage{amsmath,amsthm,amssymb,graphicx,xcolor,float,makecell,multirow}

\usepackage{esint}
\usepackage[unicode=true]{hyperref}
\hypersetup{
     colorlinks=true,       		% false: boxed links; true: colored links
     linkcolor=blue,          	% color of internal links
     citecolor=red,            % color of links to bibliography
    % filecolor=blue,      		% color of file links
     urlcolor=magenta,           	% color of external links
    % runcolor=cyan
 }

\usepackage{mathrsfs,mathtools,mathdots,dsfont}
\usepackage{listings}
\usepackage{subfigure}

%% THEOREMS -------------------------------------------------------

\newtheorem*{theorem*}{Theorem}

\newtheorem*{corollary*}{Corollary}

\newtheorem*{lemma*}{Lemma}

\newtheorem*{proposition*}{Example*}

\newtheorem*{conjecture*}{Conjecture}
\theoremstyle{definition}

\newtheorem*{definition*}{Definition}
\theoremstyle{remark}
\newtheorem{remark}{Remark}
\newtheorem*{remark*}{Remark}

\begin{document}

%\title{Exact Wave Solution For Yang-Mills Equation}

%\title{Supplemental Material for\\``General Static Solutions for the SU(2) Yang-Mills Theory''}

%\title{Exact Non-Abelian Plane Wave Solutions of the SU(2) Yang-Mills Equations}

%\title{Non-Abelian Gauge Wave: An Exact Solution of the Yang-Mills Theory}

%\title{Non-Abelian Gauge Wave: An Exact Solution of the Yang-Mills Equations}

%\title{Non-Abelian Self-Interacting Waves: Exact Solutions of the SU(2) Yang-Mills Equations}

%\title{Supplemental Material for\\``Exact SU(2) Yang-Mills Waves with Arbitrary Dispersion''}

%\title{Exactly Solving the SU(2) Yang¨CMills Equations by an Ansatz Method: Three Families of Wave Solutions}

\title{Supplemental Material for\\``Exact SU(2) Yang-Mills Waves from a Simple Ansatz''}

\author{Yu-Xuan Zhang}
\affiliation{School of Physics, Nankai University, Tianjin 300071, People's Republic of China}

\author{Jing-Ling Chen}
\email{chenjl@nankai.edu.cn}
\affiliation{Theoretical Physics Division, Chern Institute of Mathematics, Nankai University, Tianjin 300071, People's Republic of
	 	China}

\date{\today}

\begin{abstract}
\end{abstract}

%\maketitle

\maketitle\tableofcontents

\newpage

\section{The Yang-Mills Equations}

The Yang-Mills equations in vacuum without sources (i.e., the 4-vector current ${J^\nu}=0$) are given by \cite{Yang1954}
      \begin{subequations}
            \begin{align}
                  & D_\mu {F}^{\mu\nu} \equiv\partial_\mu {F}^{\mu\nu}
                        + {\rm i} g \Bigl[{A}_\mu ,\ {F}^{\mu\nu}\Bigr]=0,
                        \label{eq:YM1a} \\
                  & D_\mu {F}_{\nu\gamma} +D_\nu {F}_{\gamma\mu}
                        +D_\gamma {F}_{\mu\nu} =0. \label{eq:YM1b}
            \end{align}
      \end{subequations}
Here the covariant derivative $D_{\mu}$ is defined as
\begin{eqnarray}
D_{\mu}=\partial_{\mu}+ {\rm i} g {A}_{\mu},  \quad\;\;\;\;  (\mu=0, 1, 2, 3),
\end{eqnarray}
and the field strength tensor is
      \begin{equation}\label{eq:nonabelian}
            {F}_{\mu\nu} =\partial_\mu {A}_{\nu}
                  -\partial_\nu {A}_{\mu}
                  + {\rm i} g [{A}_{\mu},\ {A}_{\nu}], \;\;\;\;\; (\mu, \nu=0, 1, 2, 3),
      \end{equation}
where $g$ is the gauge coupling constant, the gauge potential ${A}_\mu=(\varphi, -\vec{A})$, $\varphi$ is the \emph{scalar potential}, and $\vec{A}=(A_x, A_y, A_z)$ is the \emph{vector potential}.

The matrix form of field tensor $F_{\mu\nu}$ is given by \cite{Jackson1999}
   \begin{equation}
       F_{\mu\nu}=\begin{bmatrix}
            0 & {E}_x & {E}_y & {E}_z \\
            -{E}_x & 0 & -{B}_z & {B}_y \\
            -{E}_y & {B}_z & 0 & -{B}_x \\
            -{E}_z & -{B}_y & {B}_x & 0
      \end{bmatrix},
   \end{equation}
   or
     \begin{equation}
                        {F}^{\mu\nu} =\begin{bmatrix}
                              0 & -{E}_x & -{E}_y & -{E}_z \\
                              {E}_x & 0 & -{B}_z & {B}_y \\
                              {E}_y & {B}_z & 0 & -{B}_x \\
                              {E}_z & -{B}_y & {B}_x & 0
                        \end{bmatrix}.
                  \end{equation}
Based on which, we can have the vector forms of ``magnetic'' field and ``electric'' field as
      \begin{subequations}
            \begin{eqnarray}
                  \vec{{B}} &=& \vec{\nabla}\times\vec{{A}}
                        - {\rm i} g\left(\vec{{A}}\times\vec{{A}}\right),
                      \label{eq:mag-2}  \\
                  \vec{{E}} &=& -\dfrac{1}{c}
                              \dfrac{\partial\,\vec{{A}}}{\partial\,t}
                        -\vec{\nabla}\varphi- {\rm i} g \left[\varphi,\ \vec{{A}}
                        \right], \label{eq:ele-2}
            \end{eqnarray}
      \end{subequations}
Accordingly, we can write down the Yang-Mills equations in terms of $\{\vec{B}, \vec{E}, \vec{A}, \varphi\}$ as
      \begin{subequations}
            \begin{eqnarray}
                  && \vec{\nabla}\cdot\vec{E}\ {-}\boxed{{\rm i} g\Bigl(
                        \vec{A}\cdot\vec{E}
                        -\vec{E}\cdot\vec{A}\Bigr)}=0, \label{eq:DivEYM-a} \\
                  && -\dfrac{1}{c} \dfrac{\partial \vec{B}}{\partial\,t}
                        -\vec{\nabla}\times\vec{E} {-}\boxed{{\rm i} g\biggl(\Bigl[\varphi,\
                                    \vec{B}\Bigr]
                              -\vec{A}\times\vec{E}
                              -\vec{E}\times\vec{A}\biggr)}=0, \label{eq:CurlEYM} \\
                  && \vec{\nabla}\cdot\vec{B}\ {-}\boxed{{\rm i} g\Bigl(
                        \vec{A}\cdot\vec{B}
                        -\vec{B}\cdot\vec{A}\Bigr)}=0, \label{eq:DivBYM} \\
                  && -\dfrac{1}{c} \dfrac{\partial \vec{E}}{\partial\,t}
                        +\vec{\nabla}\times\vec{B}  {-}\boxed{{\rm i} g\biggl(\Bigl[\varphi,\
                                    \vec{E}\Bigr]
                              +\vec{A}\times\vec{B}
                              +\vec{B}\times\vec{A}\biggr)}=0. \label{eq:CurlBYM-a}
            \end{eqnarray}
      \end{subequations}
Here the Yang-Mills equation (\ref{eq:YM1a}) yields Eq. (\ref{eq:DivEYM-a}) and Eq. (\ref{eq:CurlBYM-a}), the Yang-Mills equation (\ref{eq:YM1b}) is just the Bianchi identity, which yields Eq. (\ref{eq:CurlEYM}) and Eq. (\ref{eq:DivBYM}).

\begin{remark} \textcolor{blue}{The Reduction to Maxwell-Type Equations.}
If one neglects the ``boxed'' terms (or just let $g=0$), then Eqs. (\ref{eq:DivEYM-a})-(\ref{eq:CurlBYM-a}) reduce to the usual forms of Maxwell's equations (in vacuum without sources). Namely,
\begin{subequations}
            \begin{eqnarray}
                  && \vec{\nabla}\cdot\vec{{E}}=0, \label{eq:DivEYM-M} \\
                  && -\dfrac{1}{c} \dfrac{\partial \vec{{B}}}{\partial\,t}
                        -\vec{\nabla}\times\vec{{E}}=0, \label{eq:CurlEYM-M} \\
                  && \vec{\nabla}\cdot\vec{{B}}=0, \label{eq:DivBYM-M} \\
                  && -\dfrac{1}{c} \dfrac{\partial \vec{E}}{\partial\,t}
                        +\vec{\nabla}\times\vec{{B}}=0. \label{eq:CurlBYM-M}
            \end{eqnarray}
\end{subequations}
$\blacksquare$
\end{remark}

\begin{remark} \textcolor{blue}{Eq. (\ref{eq:CurlEYM}) and Eq. (\ref{eq:DivBYM}) are satisfied automatically.} Eq. (\ref{eq:CurlEYM}) and Eq. (\ref{eq:DivBYM}) are originated from the Bianchi identity (\ref{eq:YM1b}). Now we check that the Bianchi identity is automatically satisfied.
We need to prove
\begin{eqnarray}
D_\mu {F}_{\nu\gamma} + D_\nu {F}_{\gamma\mu} + D_\gamma {F}_{\mu\nu}
&=& 0,
\end{eqnarray}
Due to
\begin{eqnarray}
&& D_\mu {F}_{\nu\gamma} = [D_\mu, {F}_{\nu\gamma}], \nonumber\\
&& F_{\mu\nu} = \frac{1}{{\rm i} g} [D_\mu, D_\nu],
\end{eqnarray}
we need to prove
\begin{eqnarray}
D_\mu {F}_{\nu\gamma} + D_\nu {F}_{\gamma\mu} + D_\gamma {F}_{\mu\nu}
&=& \left[D_\mu, \left(\frac{1}{{\rm i} g} [D_\nu, D_\gamma]\right)\right]+
\left[D_\nu, \left(\frac{1}{{\rm i} g} [D_\gamma, D_\mu]\right)\right]+
\left[D_\gamma, \left(\frac{1}{{\rm i} g} [D_\mu, D_\nu]\right)\right]=0,
\end{eqnarray}
i.e.,
\begin{eqnarray}\label{jacobi}
[D_\mu, [D_\nu, D_\gamma]]+ [D_\nu, [D_\gamma, D_\mu]]+ [D_\gamma, [D_\mu, D_\nu]]=0.
\end{eqnarray}
Eq. (\ref{jacobi}) is just the Jacobi identity. This ends the proof. $\blacksquare$
\end{remark}

\begin{remark} Therefore, to find the exact solutions of the Yang-Mills equations, we only need to focus on Eq. (\ref{eq:DivEYM-a}) and Eq. (\ref{eq:CurlBYM-a}), namely,
      \begin{subequations}
            \begin{eqnarray}
                  && \vec{\nabla}\cdot\vec{E}\ {-}\boxed{{\rm i} g\Bigl(
                        \vec{A}\cdot\vec{E}
                        -\vec{E}\cdot\vec{A}\Bigr)}=0, \label{eq:DivEYM-b} \\
                  && -\dfrac{1}{c} \dfrac{\partial \vec{E}}{\partial\,t}
                        +\vec{\nabla}\times\vec{B}  {-}\boxed{{\rm i} g\biggl(\Bigl[\varphi,\
                                    \vec{E}\Bigr]
                              +\vec{A}\times\vec{B}
                              +\vec{B}\times\vec{A}\biggr)}=0, \label{eq:CurlBYM-b}
            \end{eqnarray}
      \end{subequations}
      which are the generalized Gauss's law and Ampere's law, respectively.
$\blacksquare$
\end{remark}

\section{Three Families of Exact Solutions}

\subsection{The Rotated Basis and the Ansatz}

Let $\vec{\sigma}=(\sigma_x, \sigma_y, \sigma_z)$ be the vector of Pauli's matrices. Pauli's matrices satisfy the following commutation relations:
\begin{eqnarray}
&& [\sigma_x, \sigma_y]=2{\rm i} \sigma_z, \;\;\;
[\sigma_y, \sigma_z]=2{\rm i} \sigma_x, \;\;\;
[\sigma_z, \sigma_x]=2{\rm i} \sigma_y.
\end{eqnarray}
Define a $y$-dependent rotated basis as
\begin{eqnarray}
&& \Sigma_x = \cos(\lambda y)\,\sigma_x+\sin(\lambda y)\,\sigma_y,\nonumber\\
&& \Sigma_y = -\sin(\lambda y)\,\sigma_x+\cos(\lambda y)\,\sigma_y, \nonumber\\
&&\Sigma_z = \sigma_z. 
\end{eqnarray}
It is easy to find that $\vec{\Sigma}=(\Sigma_x, \Sigma_y, \Sigma_z)$ is obtained from $\vec{\sigma}$ through a rotation in the $xy$-plane, thus one similarly has
\begin{eqnarray}
&& [\Sigma_x, \Sigma_y]=2{\rm i} \Sigma_z, \;\;\;
[\Sigma_y, \Sigma_z]=2{\rm i} \Sigma_x, \;\;\;
[\Sigma_z, \Sigma_x]=2{\rm i} \Sigma_y.
\end{eqnarray}
In this sense, one can view $\vec{\Sigma}$ as a $y$-dependent vector of Pauli's matrices. Here $\lambda$ is an arbitrary real number (ensuring $\lambda y$ is dimensionless). 

Based on which, for the vector potential and the scalar potential we set the \emph{ansatz} as
\begin{eqnarray}\label{eq:ansatz}
    \varphi &=& \alpha_1 \Sigma_x, \\
    \vec{A} &=& \alpha_2 \,\Sigma_x\, \vec{e}_z + (\alpha_3 \Sigma_z + \alpha_4 {\sin \theta}\, \Sigma_y + \alpha_5 {\cos \theta} \,\Sigma_z)\, \vec{e}_y, \nonumber
\end{eqnarray}
with the phase $\theta=kz-\omega t$, $k$ is wave number, $\omega$ is frequency, and all $\alpha_i$'s are real constants with $(i=1, 2, 3, 4, 5)$.

\subsection{Computation of $\vec{E}$ and $\vec{B}$}

 Based on Eq. (\ref{eq:ansatz}), now we can calculate the electric-like field $\vec{E}$ and the magnetic-like field.

\emph{(i) Calculation of Electric-like Field.---}Because
\begin{eqnarray}
 -\dfrac{1}{c}\dfrac{\partial\,\vec{{A}}}{\partial\,t}&=& -\dfrac{1}{c}\dfrac{\partial\, (\alpha_4 {\sin \theta}\, \Sigma_y
 + \alpha_5 {\cos \theta} \,\Sigma_z)}{\partial\,t} \vec{e}_y\nonumber\\
 &=& -\dfrac{1}{c} \left( - \omega \alpha_4 {\cos \theta}\, \Sigma_y +  \omega \alpha_5 {\sin \theta} \,\Sigma_z \right) \vec{e}_y, \nonumber\\
 &=& \frac{\omega}{c} \left( \alpha_4 {\cos \theta}\, \Sigma_y -\alpha_5 {\sin \theta} \,\Sigma_z \right) \vec{e}_y\nonumber\\
 -\vec{\nabla}\varphi &=& -\frac{\partial \left(\alpha_1 \Sigma_x\right)}{\partial y} \vec{e}_y = -\alpha_1 \frac{\partial \Sigma_x}{\partial y} \vec{e}_y  = - \lambda \alpha_1 \Sigma_y \vec{e}_y,  \nonumber\\
 - {\rm i} g \left[\varphi,\ \vec{A} \right]&=& - {\rm i} g \left[\alpha_1 \Sigma_x,\ \alpha_3 \Sigma_z + \alpha_4 {\sin \theta}\, \Sigma_y + \alpha_5 {\cos \theta} \,\Sigma_z\right] \vec{e}_y \nonumber\\
&=& - {\rm i} g (2 {\rm i}) \alpha_1 \left( -\alpha_3 \Sigma_y + \alpha_4 {\sin \theta}\, \Sigma_z - \alpha_5 {\cos \theta} \,\Sigma_y\right) \vec{e}_y \nonumber\\
&=& 2 g \alpha_1 \left( -\alpha_3 \Sigma_y + \alpha_4 {\sin \theta}\, \Sigma_z - \alpha_5 {\cos \theta} \,\Sigma_y\right) \vec{e}_y,
\end{eqnarray}
then we have
\begin{eqnarray}\label{eq:E-a}
\vec{{E}}&=& -\dfrac{1}{c}\dfrac{\partial\,\vec{{A}}}{\partial\,t}
-\vec{\nabla}\varphi- {\rm i} g \left[\varphi,\ \vec{{A}}\right]\nonumber\\
&=&  \frac{\omega}{c} \left( \alpha_4 {\cos \theta}\, \Sigma_y -\alpha_5 {\sin \theta} \,\Sigma_z \right) \vec{e}_y
\textcolor{black}{- \lambda \alpha_1 \Sigma_y \vec{e}_y}
+ 2 g \alpha_1 \left( -\alpha_3 \Sigma_y + \alpha_4 {\sin \theta}\, \Sigma_z - \alpha_5 {\cos \theta} \,\Sigma_y\right) \vec{e}_y\nonumber\\
&=&   \left[ \left( \textcolor{black}{- \lambda \alpha_1}-  2g \alpha_1\alpha_3 + \frac{\omega}{c}  \alpha_4 {\cos \theta} - 2g \alpha_1\alpha_5 {\cos \theta}  \right) \Sigma_y
+\left(-\frac{\omega}{c} \alpha_5 {\sin \theta} + 2 g \alpha_1 \alpha_4 {\sin \theta} \right) \Sigma_z \right] \vec{e}_y\nonumber\\
&=&   \left\{ \left[ (\textcolor{black}{- \lambda \alpha_1}-  2g \alpha_1\alpha_3) + \left(\frac{\omega}{c}  \alpha_4  - 2g \alpha_1\alpha_5\right) {\cos \theta}  \right] \Sigma_y
+\left(-\frac{\omega}{c} \alpha_5  + 2 g \alpha_1 \alpha_4  \right){\sin \theta} \Sigma_z \right\} \vec{e}_y.
\end{eqnarray}

\emph{(ii) Calculation of Magnetic-like Field.---}Because

\begin{eqnarray}
\vec{\nabla}\times\vec{{A}} &=& \left(\frac{\partial A_z}{\partial y}-\frac{\partial A_y}{\partial z}\right)\vec{e}_x+
\left(\frac{\partial A_x}{\partial z}-\frac{\partial A_z}{\partial x}\right)\vec{e}_y+
\left(\frac{\partial A_y}{\partial x}-\frac{\partial A_x}{\partial y}\right)\vec{e}_z= \left(\frac{\partial A_z}{\partial y}-\frac{\partial A_y}{\partial z}\right)\vec{e}_x \nonumber\\
&=& \left[ \frac{\partial (\alpha_2 \,\Sigma_x)}{\partial y}-\frac{\partial (\alpha_3 \Sigma_z + \alpha_4 {\sin \theta}\, \Sigma_y + \alpha_5 {\cos \theta}\,\Sigma_z)}{\partial z} \right]\vec{e}_x \nonumber\\
&=& \left\{ \lambda \alpha_2 \left[-\sin (\lambda y)\,\sigma_x + \cos (\lambda y)\,\sigma_y\right]
- k(\alpha_4 {\cos \theta}\, \Sigma_y - \alpha_5 {\sin \theta}\,\Sigma_z)\right\}\vec{e}_x \nonumber\\
&=&  \left[\lambda \alpha_2 \Sigma_y -k\alpha_4 {\cos \theta}\, \Sigma_y + k \alpha_5 {\sin \theta}\,\Sigma_z\right]\; \vec{e}_x, \nonumber\\
- {\rm i} g\left(\vec{{A}}\times\vec{{A}}\right) &=& - {\rm i} g \left\{ [A_y, A_z] \vec{e}_x +  [A_z, A_x] \vec{e}_y + [A_x, A_y] \vec{e}_z\right\} = - {\rm i} g [A_y, A_z] \vec{e}_x \nonumber\\
 &=& - {\rm i} g [\alpha_3 \Sigma_z + \alpha_4 {\sin \theta}\, \Sigma_y + \alpha_5 {\cos \theta} \,\Sigma_z,\;  \alpha_2 \,\Sigma_x] \vec{e}_x \nonumber\\
 &=& - {\rm i} g (2{\rm i}) \alpha_2 \left(\alpha_3 \Sigma_y - \alpha_4 {\sin \theta}\, \Sigma_z + \alpha_5 {\cos \theta} \,\Sigma_y\right) \vec{e}_x \nonumber\\
 &=& 2g \alpha_2 \left(\alpha_3 \Sigma_y - \alpha_4 {\sin \theta}\, \Sigma_z + \alpha_5 {\cos \theta} \,\Sigma_y\right) \vec{e}_x,
\end{eqnarray}
then we have
\begin{eqnarray}
\vec{{B}} &=& \vec{\nabla}\times\vec{{A}}- {\rm i} g\left(\vec{{A}}\times\vec{{A}}\right) \nonumber\\
&=& \left[\lambda \alpha_2 \Sigma_y -k\alpha_4 {\cos \theta}\, \Sigma_y + k \alpha_5 {\sin \theta}\,\Sigma_z\right]\; \vec{e}_x +
2g \alpha_2 \left(\alpha_3 \Sigma_y - \alpha_4 {\sin \theta}\, \Sigma_z + \alpha_5 {\cos \theta} \,\Sigma_y\right) \vec{e}_x \nonumber\\
&=& \left[ \left(\lambda \alpha_2 -k\alpha_4 {\cos \theta} + 2g \alpha_2 \alpha_3 + 2 g \alpha_2 \alpha_5 {\cos \theta} \right)\Sigma_y +\left[ k \alpha_5 {\sin \theta}- 2g \alpha_2 \alpha_4 {\sin \theta}\right]\, \Sigma_z \right]\vec{e}_x\nonumber\\
&=& \left\{ \left[ (\lambda \alpha_2 + 2g \alpha_2 \alpha_3)+ \left( -k\alpha_4  + 2 g \alpha_2 \alpha_5 \right){\cos \theta} \right]\Sigma_y +\left( k \alpha_5 - 2g \alpha_2 \alpha_4 \right){\sin \theta}\, \Sigma_z \right\}\vec{e}_x.
\end{eqnarray}

\subsection{Computation of the Generalized Gauss's Law and Amp{\`e}re's Law}

\emph{(i) Calculation of the Generalized Gauss's Law, i.e., Eq. (\ref{eq:DivEYM-b}).---}Because

\begin{eqnarray}
&& \frac{\partial \Sigma_x}{\partial y} =\lambda \Sigma_y, \;\;\;\;  \frac{\partial \Sigma_y}{\partial y} =-\lambda \Sigma_x,
\end{eqnarray}

\begin{eqnarray}
\vec{\nabla}\cdot\vec{E} &=&  \frac{\partial}{\partial y}   \left\{ \left[ (\textcolor{black}{- \lambda \alpha_1}-  2g \alpha_1\alpha_3) + \left(\frac{\omega}{c}  \alpha_4  - 2g \alpha_1\alpha_5\right) {\cos \theta}  \right] \Sigma_y
+\left(-\frac{\omega}{c} \alpha_5  + 2 g \alpha_1 \alpha_4  \right){\sin \theta} \Sigma_z \right\}\nonumber\\
 &=&  \left[ (\textcolor{black}{- \lambda \alpha_1}-  2g \alpha_1\alpha_3) + \left(\frac{\omega}{c}  \alpha_4  - 2g \alpha_1\alpha_5\right) {\cos \theta}  \right] \frac{\partial \Sigma_y}{\partial y}   \nonumber\\
% &=&  -\lambda
% \left[ (\textcolor{black}{- \lambda \alpha_1}-  2g \alpha_1\alpha_3) + \left(\frac{\omega}{c}  \alpha_4  - 2g \alpha_1\alpha_5\right) {\cos \theta}  \right] \Sigma_x\nonumber\\
&=&
 \left[ \lambda(\textcolor{black}{ \lambda \alpha_1} + 2g \alpha_1\alpha_3) -\lambda \left(\frac{\omega}{c}  \alpha_4  - 2g \alpha_1\alpha_5\right) {\cos \theta}  \right] \Sigma_x,
\end{eqnarray}

\begin{eqnarray}
 && -{\rm i} g\left( \vec{A}\cdot\vec{E} -\vec{E}\cdot\vec{A}\right) \nonumber\\
 &=&
 -{\rm i} g\left[(\alpha_3+ \alpha_5 {\cos \theta})\Sigma_z + \alpha_4 {\sin \theta}\, \Sigma_y, \;
  E_y \right]\nonumber\\
 &=&
 -{\rm i} g\left[(\alpha_3+ \alpha_5 {\cos \theta})\Sigma_z, \;
  \left[ (\textcolor{black}{- \lambda \alpha_1}-  2g \alpha_1\alpha_3) + \left(\frac{\omega}{c}  \alpha_4  - 2g \alpha_1\alpha_5\right) {\cos \theta}  \right] \Sigma_y \right]\nonumber\\
&& -{\rm i} g\left[\alpha_4 {\sin \theta}\, \Sigma_y, \;
 \left(-\frac{\omega}{c} \alpha_5  + 2 g \alpha_1 \alpha_4  \right){\sin \theta} \Sigma_z\right]\nonumber\\
 &=&
 -{\rm i} g (2{\rm i}) \left[-(\alpha_3+ \alpha_5 {\cos \theta})
  \left[ (\textcolor{black}{- \lambda \alpha_1}-  2g \alpha_1\alpha_3) + \left(\frac{\omega}{c}  \alpha_4  - 2g \alpha_1\alpha_5\right) {\cos \theta}  \right]
  + \alpha_4 {\sin \theta} \left(-\frac{\omega}{c} \alpha_5  + 2 g \alpha_1 \alpha_4  \right){\sin \theta}\right]\Sigma_x \nonumber\\
 &=&
 2 g \left\{(\alpha_3+ \alpha_5 {\cos \theta})
  \left[  (\textcolor{black}{ \lambda \alpha_1}+ 2g \alpha_1\alpha_3) -\left( \frac{\omega}{c}  \alpha_4  - 2g \alpha_1\alpha_5 \right){\cos \theta}\right]
+ \alpha_4 \left(-\frac{\omega}{c} \alpha_5 + 2 g \alpha_1 \alpha_4 \right){\sin^2 \theta}\right\}\Sigma_x \nonumber\\
 &=&
 2 g \left\{(\alpha_3+ \alpha_5 {\cos \theta})
  \left[ (\textcolor{black}{ \lambda \alpha_1}+ 2g \alpha_1\alpha_3) -\left( \frac{\omega}{c}  \alpha_4  - 2g \alpha_1\alpha_5 \right){\cos \theta}\right]
+ \alpha_4 \left(-\frac{\omega}{c} \alpha_5 + 2 g \alpha_1 \alpha_4 \right)\left(1-{\cos^2 \theta}\right)\right\}\Sigma_x \nonumber\\
 &=&
 2 g \biggr\{ \left[\alpha_3 (\textcolor{black}{ \lambda \alpha_1}+ 2g \alpha_1\alpha_3) + \alpha_4 \left(-\frac{\omega}{c} \alpha_5 + 2 g \alpha_1 \alpha_4 \right) \right]
 +\left[-\alpha_3 \left( \frac{\omega}{c}  \alpha_4  - 2g \alpha_1\alpha_5 \right)+ \alpha_5 (\textcolor{black}{ \lambda \alpha_1}+ 2g \alpha_1\alpha_3) \right]{\cos \theta} \nonumber\\
   && {-} \left[\alpha_5 \left( \frac{\omega}{c}  \alpha_4  - 2g \alpha_1\alpha_5 \right) +\alpha_4 \left(-\frac{\omega}{c} \alpha_5 + 2 g \alpha_1 \alpha_4 \right)\right]{\cos^2 \theta} \biggr\}\Sigma_x \nonumber\\
 &=&
 2 g \biggr\{ \left[ \textcolor{black}{ \lambda \alpha_1}\alpha_3 -\frac{\omega}{c} \alpha_4 \alpha_5 + 2 g \alpha_1(\alpha_3^2+\alpha_4^2) \right]
 +\left[  \textcolor{black}{ \lambda \alpha_1}\alpha_5 - \frac{\omega}{c} \alpha_3 \alpha_4 + 4g \alpha_1\alpha_3 \alpha_5 \right]{\cos \theta}
 {-} 2g \alpha_1(\alpha_4^2-\alpha_5^2) {\cos^2 \theta} \biggr\}\Sigma_x.
\end{eqnarray}
Then from Eq. (\ref{eq:DivEYM-b}) we have
\begin{eqnarray}\label{eq:analy-1}
 && \vec{\nabla}\cdot\vec{E} -{\rm i} g\Bigl(\vec{A}\cdot\vec{E}-\vec{E}\cdot\vec{A}\Bigr)\nonumber\\
&=&
 \left[ \lambda(\textcolor{black}{ \lambda \alpha_1} + 2g \alpha_1\alpha_3) -\lambda \left(\frac{\omega}{c}  \alpha_4  - 2g \alpha_1\alpha_5\right) {\cos \theta}  \right] \Sigma_x \nonumber\\
&&
 +2 g \biggr\{ \left[ \textcolor{black}{ \lambda \alpha_1}\alpha_3 -\frac{\omega}{c} \alpha_4 \alpha_5 + 2 g \alpha_1(\alpha_3^2+\alpha_4^2) \right]
 +\left[  \textcolor{black}{ \lambda \alpha_1}\alpha_5 - \frac{\omega}{c} \alpha_3 \alpha_4 + 4g \alpha_1\alpha_3 \alpha_5 \right]{\cos \theta}
 {-} 2g \alpha_1(\alpha_4^2-\alpha_5^2) {\cos^2 \theta} \biggr\}\Sigma_x \nonumber\\
&=&
 \left\{ \left[\alpha_1(\lambda + 2g\alpha_3)^2 + 2g\alpha_4\left(2g\alpha_1\alpha_4 - \frac{\omega}{c}\alpha_5\right)\right]+(\lambda + 2g\alpha_3)\left(4g\alpha_1\alpha_5 - \frac{\omega}{c}\alpha_4\right){\cos \theta} -4g^2 \alpha_1(\alpha_4^2 - \alpha_5^2) {\cos^2 \theta} \right\} \Sigma_x \nonumber\\
&=& 0.
\end{eqnarray}

\emph{(ii) Calculation of the Generalized Amp{\`e}re's Law, i.e., Eq. (\ref{eq:CurlBYM-b}).---}Because

\begin{eqnarray}
 -\dfrac{1}{c} \dfrac{\partial \vec{E}}{\partial\,t}
 &=&  -\dfrac{1}{c} \dfrac{\partial \left\{ \left[ (\textcolor{black}{- \lambda \alpha_1}-  2g \alpha_1\alpha_3) + \left(\frac{\omega}{c}  \alpha_4  - 2g \alpha_1\alpha_5\right) {\cos \theta}  \right] \Sigma_y
+\left(-\frac{\omega}{c} \alpha_5  + 2 g \alpha_1 \alpha_4  \right){\sin \theta} \Sigma_z \right\} }{\partial\,t} \vec{e}_y \nonumber\\
 &=&  -\dfrac{1}{c} \left\{ \left[ \omega \left(\frac{\omega}{c}  \alpha_4  - 2g \alpha_1\alpha_5\right) {\sin \theta}  \right] \Sigma_y
-\omega\left(-\frac{\omega}{c} \alpha_5  + 2 g \alpha_1 \alpha_4  \right){\cos \theta} \Sigma_z \right\} \vec{e}_y \nonumber\\
 &=&  \left[ - \frac{\omega}{c} \left(\frac{\omega}{c}  \alpha_4  - 2g \alpha_1\alpha_5\right) {\sin \theta} \; \Sigma_y
 +\frac{\omega}{c}\left(-\frac{\omega}{c} \alpha_5  + 2 g \alpha_1 \alpha_4  \right){\cos \theta}\; \Sigma_z \right] \vec{e}_y,
\end{eqnarray}

\begin{eqnarray}
\vec{\nabla}\times\vec{B}
&=& \left(\frac{\partial B_z}{\partial y}-\frac{\partial B_y}{\partial z}\right)\vec{e}_x+
\left(\frac{\partial B_x}{\partial z}-\frac{\partial B_z}{\partial x}\right)\vec{e}_y+
\left(\frac{\partial B_y}{\partial x}-\frac{\partial B_x}{\partial y}\right)\vec{e}_z\nonumber\\
&=& \frac{\partial B_x}{\partial z} \vec{e}_y-\frac{\partial B_x}{\partial y} \vec{e}_z\nonumber\\
&=& \frac{\partial \left\{ \left[ (\lambda \alpha_2 + 2g \alpha_2 \alpha_3)+ \left( -k\alpha_4  + 2 g \alpha_2 \alpha_5 \right){\cos \theta} \right]\Sigma_y +\left( k \alpha_5 - 2g \alpha_2 \alpha_4 \right){\sin \theta}\, \Sigma_z \right\}}{\partial z} \vec{e}_y \nonumber\\
&&-\frac{\partial \left\{ \left[ (\lambda \alpha_2 + 2g \alpha_2 \alpha_3)+ \left( -k\alpha_4  + 2 g \alpha_2 \alpha_5 \right){\cos \theta} \right]\Sigma_y +\left( k \alpha_5 - 2g \alpha_2 \alpha_4 \right){\sin \theta}\, \Sigma_z \right\} }{\partial y} \vec{e}_z\nonumber\\
&=& \left\{ \left[ -k \left( -k\alpha_4  + 2 g \alpha_2 \alpha_5 \right){\sin \theta} \right]\Sigma_y +k \left( k \alpha_5 - 2g \alpha_2 \alpha_4 \right){\cos \theta}\, \Sigma_z \right\} \vec{e}_y \nonumber\\
&&- \left\{ \left[ (\lambda \alpha_2 + 2g \alpha_2 \alpha_3)+ \left( -k\alpha_4  + 2 g \alpha_2 \alpha_5 \right){\cos \theta} \right]
(-\lambda \Sigma_x) \right\} \vec{e}_z\nonumber\\
&=& k \left[ \left( k\alpha_4  - 2 g \alpha_2 \alpha_5 \right){\sin \theta} \Sigma_y + \left( k \alpha_5 - 2g \alpha_2 \alpha_4 \right){\cos \theta}\, \Sigma_z \right] \vec{e}_y \nonumber\\
&&+\lambda  \left[ (\lambda \alpha_2 + 2g \alpha_2 \alpha_3)+ \left( -k\alpha_4  + 2 g \alpha_2 \alpha_5 \right){\cos \theta} \right]
\Sigma_x  \vec{e}_z,
\end{eqnarray}

\begin{eqnarray}
-{\rm i} g \left[\varphi,\, \vec{E}\right]
&=& -{\rm i} g \left[\alpha_1 \Sigma_x,\,   \left[ (\textcolor{black}{- \lambda \alpha_1}-  2g \alpha_1\alpha_3) + \left(\frac{\omega}{c}  \alpha_4  - 2g \alpha_1\alpha_5\right) {\cos \theta}  \right] \Sigma_y
+\left(-\frac{\omega}{c} \alpha_5  + 2 g \alpha_1 \alpha_4  \right){\sin \theta} \Sigma_z   \right] \vec{e}_y \nonumber\\
&=& -{\rm i} g (2{\rm i}) \alpha_1 \left\{ \left[ (\textcolor{black}{- \lambda \alpha_1}-  2g \alpha_1\alpha_3) + \left(\frac{\omega}{c}  \alpha_4  - 2g \alpha_1\alpha_5\right) {\cos \theta}  \right]  \Sigma_z
-\left(-\frac{\omega}{c} \alpha_5  + 2 g \alpha_1 \alpha_4  \right){\sin \theta} \Sigma_y  \right\} \vec{e}_y \nonumber\\
&=& 2g \alpha_1 \left\{ \left[ (\textcolor{black}{- \lambda \alpha_1}-  2g \alpha_1\alpha_3) + \left(\frac{\omega}{c}  \alpha_4  - 2g \alpha_1\alpha_5\right) {\cos \theta}  \right]  \Sigma_z
-\left(-\frac{\omega}{c} \alpha_5  + 2 g \alpha_1 \alpha_4  \right){\sin \theta} \Sigma_y  \right\} \vec{e}_y,
\end{eqnarray}

\begin{eqnarray}
&&{\rm i} g \left[A_y, \; B_x \right] \nonumber\\
&=& {\rm i} g \left[ (\alpha_3 + \alpha_5 {\cos \theta})\Sigma_z + \alpha_4 {\sin \theta}\, \Sigma_y,
\;   \left[ (\lambda \alpha_2 + 2g \alpha_2 \alpha_3)+ \left( -k\alpha_4  + 2 g \alpha_2 \alpha_5 \right){\cos \theta} \right]\Sigma_y +\left( k \alpha_5 - 2g \alpha_2 \alpha_4 \right){\sin \theta}\, \Sigma_z  \right] \nonumber\\
&=& {\rm i} g (2 {\rm i}) \left\{ -(\alpha_3 + \alpha_5 {\cos \theta}) [(\lambda \alpha_2 + 2g \alpha_2 \alpha_3)+ \left( -k\alpha_4  + 2 g \alpha_2 \alpha_5 \right){\cos \theta}] + \alpha_4 {\sin \theta}\left( k \alpha_5 - 2g \alpha_2 \alpha_4 \right){\sin \theta} \right\} \, \Sigma_x \nonumber\\
&=& -2 g  \left\{ -(\alpha_3 + \alpha_5 {\cos \theta}) [(\lambda \alpha_2 + 2g \alpha_2 \alpha_3)+ \left( -k\alpha_4  + 2 g \alpha_2 \alpha_5 \right){\cos \theta}] + \alpha_4 \left( k \alpha_5 - 2g \alpha_2 \alpha_4 \right){\sin^2 \theta} \right\} \, \Sigma_x \nonumber\\
&=& 2 g  \left\{ (\alpha_3 + \alpha_5 {\cos \theta}) [(\lambda \alpha_2 + 2g \alpha_2 \alpha_3)+ \left( -k\alpha_4  + 2 g \alpha_2 \alpha_5 \right){\cos \theta}] - \alpha_4 \left( k \alpha_5 - 2g \alpha_2 \alpha_4 \right){\sin^2 \theta} \right\} \, \Sigma_x \nonumber\\
&=& 2 g  \left\{ (\alpha_3 + \alpha_5 {\cos \theta}) [(\lambda \alpha_2 + 2g \alpha_2 \alpha_3)+ \left( -k\alpha_4  \textcolor{black}{+} 2 g \alpha_2 \alpha_5 \right){\cos \theta}] - \alpha_4 \left( k \alpha_5 - 2g \alpha_2 \alpha_4 \right) (1-{\cos^2 \theta}) \right\} \, \Sigma_x \nonumber\\
&=& 2 g  \biggr\{
[\alpha_3(\lambda \alpha_2 + 2g \alpha_2 \alpha_3)- \alpha_4 \left( k \alpha_5 - 2g \alpha_2 \alpha_4 \right)] \nonumber\\
&&+[\alpha_3 \left( -k\alpha_4  \textcolor{black}{+} 2 g \alpha_2 \alpha_5 \right)+  \alpha_5 (\lambda \alpha_2 + 2g \alpha_2 \alpha_3)]{\cos \theta}
 + \left[ \textcolor{black}{\alpha_5\left( -k\alpha_4  \textcolor{black}{+} 2 g \alpha_2 \alpha_5 \right)}+\alpha_4 \left( k \alpha_5 - 2g \alpha_2 \alpha_4 \right)\right]{\cos^2 \theta} \biggr\} \, \Sigma_x \nonumber\\
&=& 2 g  \biggr\{
[ \lambda \alpha_2 \alpha_3 -k \alpha_4 \alpha_5 + 2g \alpha_2 (\alpha_3^2+\alpha_4^2)] +(\lambda \alpha_2 \alpha_5 - k \alpha_3 \alpha_4 \textcolor{black}{+4 g\alpha_2\alpha_3\alpha_5} ){\cos \theta}
 \textcolor{black}{+ 2g\alpha_2 \left( \alpha_5^2 - \alpha_4^2 \right)}{\cos^2 \theta} \biggr\} \, \Sigma_x,
\end{eqnarray}

\begin{eqnarray}
&&-{\rm i} g \left[A_z, \; B_x \right] \nonumber\\
&=& -{\rm i} g \left[\alpha_2 \,\Sigma_x, \;  \left[ (\lambda \alpha_2 + 2g \alpha_2 \alpha_3)+ \left( -k\alpha_4  + 2 g \alpha_2 \alpha_5 \right){\cos \theta} \right]\Sigma_y +\left( k \alpha_5 - 2g \alpha_2 \alpha_4 \right){\sin \theta}\, \Sigma_z \right] \nonumber\\
&=& -{\rm i} g (2 {\rm i}) \alpha_2 \left\{ \left[ (\lambda \alpha_2 + 2g \alpha_2 \alpha_3)+ \left( -k\alpha_4  + 2 g \alpha_2 \alpha_5 \right){\cos \theta} \right]\Sigma_z -\left( k \alpha_5 - 2g \alpha_2 \alpha_4 \right){\sin \theta}\, \Sigma_y \right\}\nonumber\\
&=& 2g \alpha_2 \left\{ \left[ (\lambda \alpha_2 + 2g \alpha_2 \alpha_3)+ \left( -k\alpha_4  + 2 g \alpha_2 \alpha_5 \right){\cos \theta} \right]\Sigma_z -\left( k \alpha_5 - 2g \alpha_2 \alpha_4 \right){\sin \theta}\, \Sigma_y \right\},
\end{eqnarray}

\begin{eqnarray}
&& -{\rm i} g \left(\vec{A}\times\vec{B}+\vec{B}\times\vec{A}\right)\nonumber\\
&=&  -{\rm i} g \left[ \left(A_y \vec{e}_y+A_z \vec{e}_z\right) \times B_x \vec{e}_x + B_x \vec{e}_x\times \left(A_y \vec{e}_y+A_z \vec{e}_z\right) \right] \nonumber\\
&=&  -{\rm i} g \left(  -A_y B_x \vec{e}_z+A_z B_x \vec{e}_y + B_x A_y  \vec{e}_z - B_x A_z \vec{e}_y \right) \nonumber\\
&=&  {\rm i} g \left[A_y, B_x \right] \textcolor{black}{\vec{e}_z} - {\rm i} g \left[A_z, B_x \right] \textcolor{black}{\vec{e}_y} \nonumber\\
&=& 2 g  \biggr\{
[ \lambda \alpha_2 \alpha_3 -k \alpha_4 \alpha_5 + 2g \alpha_2 (\alpha_3^2+\alpha_4^2)] +(\lambda \alpha_2 \alpha_5 - k \alpha_3 \alpha_4 \textcolor{black}{+4 g\alpha_2\alpha_3\alpha_5} ){\cos \theta}
 \textcolor{black}{+ 2g\alpha_2 \left( \alpha_5^2 - \alpha_4^2 \right)}{\cos^2 \theta} \biggr\} \, \Sigma_x\, \textcolor{black}{\vec{e}_z}  \nonumber\\
 &&+ 2g \alpha_2 \left\{ \left[ (\lambda \alpha_2 + 2g \alpha_2 \alpha_3)+ \left( -k\alpha_4  + 2 g \alpha_2 \alpha_5 \right){\cos \theta} \right]\Sigma_z -\left( k \alpha_5 - 2g \alpha_2 \alpha_4 \right){\sin \theta}\, \Sigma_y \right\} \textcolor{black}{\vec{e}_y},
\end{eqnarray}
then we have

\begin{eqnarray}\label{eq:analy-2}
&& -\dfrac{1}{c} \dfrac{\partial \vec{E}}{\partial\,t}
                        +\vec{\nabla}\times\vec{B}  {-}{\rm i} g\biggl(\Bigl[\varphi,\
                                    \vec{E}\Bigr]
                              +\vec{A}\times\vec{B}
                              +\vec{B}\times\vec{A}\biggr)\nonumber\\
&=& \left[ - \frac{\omega}{c} \left(\frac{\omega}{c}  \alpha_4  - 2g \alpha_1\alpha_5\right) {\sin \theta} \; \Sigma_y
 +\frac{\omega}{c}\left(-\frac{\omega}{c} \alpha_5  + 2 g \alpha_1 \alpha_4  \right){\cos \theta}\; \Sigma_z \right] \vec{e}_y \nonumber\\
&&+ k \left[ \left( k\alpha_4  - 2 g \alpha_2 \alpha_5 \right){\sin \theta} \Sigma_y + \left( k \alpha_5 - 2g \alpha_2 \alpha_4 \right){\cos \theta}\, \Sigma_z \right] \vec{e}_y \nonumber\\
&&+\lambda  \left[ (\lambda \alpha_2 + 2g \alpha_2 \alpha_3)+ \left( -k\alpha_4  + 2 g \alpha_2 \alpha_5 \right){\cos \theta} \right]
\Sigma_x  \vec{e}_z\nonumber\\
&&+ 2g \alpha_1 \left\{ \left[ (\textcolor{black}{- \lambda \alpha_1}-  2g \alpha_1\alpha_3) + \left(\frac{\omega}{c}  \alpha_4  - 2g \alpha_1\alpha_5\right) {\cos \theta}  \right]  \Sigma_z
-\left(-\frac{\omega}{c} \alpha_5  + 2 g \alpha_1 \alpha_4  \right){\sin \theta} \Sigma_y  \right\} \vec{e}_y\nonumber\\
&&+ 2 g  \biggr\{
[ \lambda \alpha_2 \alpha_3 -k \alpha_4 \alpha_5 + 2g \alpha_2 (\alpha_3^2+\alpha_4^2)] +(\lambda \alpha_2 \alpha_5 - k \alpha_3 \alpha_4 \textcolor{black}{+4 g\alpha_2\alpha_3\alpha_5} ){\cos \theta}
 \textcolor{black}{+ 2g\alpha_2 \left( \alpha_5^2 - \alpha_4^2 \right)}{\cos^2 \theta} \biggr\} \, \Sigma_x\, \textcolor{black}{\vec{e}_z}  \nonumber\\
 &&+ 2g \alpha_2 \left\{ \left[ (\lambda \alpha_2 + 2g \alpha_2 \alpha_3)+ \left( -k\alpha_4  + 2 g \alpha_2 \alpha_5 \right){\cos \theta} \right]\Sigma_z -\left( k \alpha_5 - 2g \alpha_2 \alpha_4 \right){\sin \theta}\, \Sigma_y \right\} \textcolor{black}{\vec{e}_y}=0,
 \end{eqnarray}
i.e.,
\begin{eqnarray}\label{eq:analy-2}
&& -\dfrac{1}{c} \dfrac{\partial \vec{E}}{\partial\,t}
                        +\vec{\nabla}\times\vec{B}  {-}{\rm i} g\biggl(\Bigl[\varphi,\
                                    \vec{E}\Bigr]
                              +\vec{A}\times\vec{B}
                              +\vec{B}\times\vec{A}\biggr)\nonumber\\
&=& \biggr\{ 2g\left[(\alpha_2^2 - \alpha_1^2)(\lambda + 2g\alpha_3) \right]\Sigma_z + \left[\alpha_5\left(k^2 - \frac{\omega^2}{c^2} - 4g^2(\alpha_1^2 - \alpha_2^2)\right) + 4g\alpha_4\left(\frac{\omega}{c}\alpha_1 - k\alpha_2\right)\right]{\cos \theta} \Sigma_z \nonumber\\
&& +  \left[\alpha_4\left(k^2 - \frac{\omega^2}{c^2} - 4g^2(\alpha_1^2 - \alpha_2^2)\right) + 4g\alpha_5\left(\frac{\omega}{c}\alpha_1 - k\alpha_2\right)\right]{\sin \theta}\Sigma_y  \biggr\} \vec{e}_y \nonumber\\
&&+ {\Bigg\{ \Big[\alpha_2(\lambda+2g\alpha_3)^2 + 2g\alpha_4(2g\alpha_2\alpha_4 - k\alpha_5)\Big]  + \Big[(\lambda+2g\alpha_3)(4g\alpha_2\alpha_5 - k\alpha_4)\Big]\cos\theta} \nonumber\\
&&+ { 4g^2\alpha_2(\alpha_5^2-\alpha_4^2)\cos^2\theta \Bigg\}\, \Sigma_x \vec{e}_z}=0.
\end{eqnarray}

%\begin{eqnarray}
%&-\frac{1}{c}\frac{\partial\vec{E}}{\partial t} + \vec{\nabla}\times \vec{B} - \mathrm{i}g\Big([\phi,\vec{E}] + \vec{A}\times\vec{B} + \vec{B}\times\vec{A}\Big) \\
%&= \Bigg\{ 2g(\alpha_2^2-\alpha_1^2)(\lambda+2g\alpha_3)\,\Sigma_z \\
%&\quad + \Big[\alpha_5\Big(k^2-\frac{\omega^2}{c^2}-4g^2(\alpha_1^2-\alpha_2^2)\Big) + 4g\alpha_4\Big(\frac{\omega}{c}\alpha_1 - k\alpha_2\Big)\Big]\cos\theta\,\Sigma_z \\
%&\quad + \Big[\alpha_4\Big(k^2-\frac{\omega^2}{c^2}-4g^2(\alpha_1^2-\alpha_2^2)\Big) + 4g\alpha_5\Big(\frac{\omega}{c}\alpha_1 - k\alpha_2\Big)\Big]\sin\theta\,\Sigma_y \Bigg\} \vec{e}_y \\
%&\quad + \Bigg\{ \Big[\alpha_2(\lambda+2g\alpha_3)^2 + 2g\alpha_4(2g\alpha_2\alpha_4 - k\alpha_5)\Big] \\
%&\quad + \Big[(\lambda+2g\alpha_3)(4g\alpha_2\alpha_5 - k\alpha_4)\Big]\cos\theta \\
%&\quad + 4g^2\alpha_2(\alpha_5^2-\alpha_4^2)\cos^2\theta \Bigg\} \Sigma_x\,\vec{e}_z .
%\end{eqnarray}

\subsection{Nine Algebraic Constraints from Eq. (\ref{eq:analy-1}) and Eq. (\ref{eq:analy-2})}

In this work, we focus on the nontrivial case of $g\neq 0$. In the following, let us come to analyze Eq. (\ref{eq:analy-1}) and Eq. (\ref{eq:analy-2}). Firstly, we show that the case of $k=0$ and $\omega=0$ is trivial.

\begin{remark} \textcolor{blue}{The case of $k=0$ and $\omega=0$ is trivial.} In this case, one has $\theta=kz -\omega t=0$, $\cos\theta=1$, $\sin\theta=0$, and evidently the scalar potential $\varphi$ and the vector potential $\vec{A}$ do not depend on time $t$. Then one has
\begin{eqnarray}
 && \vec{\nabla}\cdot\vec{E} -{\rm i} g\Bigl(\vec{A}\cdot\vec{E}-\vec{E}\cdot\vec{A}\Bigr)
= \alpha_1 [\lambda+ 2g (\alpha_3+\alpha_5)]^2 \Sigma_x=0,
\end{eqnarray}

\begin{eqnarray}
&&-\frac{1}{c}\frac{\partial\vec{E}}{\partial t} +\vec{\nabla}\times \vec{B} -\mathrm{i}g\Big([\phi,\vec{E}]+\vec{A}\times\vec{B}+\vec{B}\times\vec{A}\Big) \nonumber\\
&=& -2g(\alpha_1^2-\alpha_2^2)\big(\lambda+2g(\alpha_3+\alpha_5)\big)\Sigma_z\vec{e}_y + \alpha_2\big(\lambda+2g(\alpha_3+\alpha_5)\big)^2\Sigma_x\vec{e}_z = 0.
\end{eqnarray}
By considering $g \neq 0$, we then have three constraint equations:
\begin{eqnarray}
&& \alpha_1 [\lambda+ 2g (\alpha_3+\alpha_5)]^2=0,\nonumber\\
&& (\alpha_1^2  - \alpha_2^2  )\left[\lambda  +2 g  (\alpha_3 +\alpha_5) \right]=0, \nonumber\\
&& \alpha_2\big(\lambda+2g(\alpha_3+\alpha_5)\big)^2=0,
\end{eqnarray}
which leads to (i) $[\lambda+ 2g (\alpha_3+\alpha_5)]=0$ and (ii) $\{\alpha_1=0, \alpha_2=0\}$.
Accordingly, we have the electric-like field and the magnetic-like field as
\begin{eqnarray}
\vec{{E}} &=&   \left\{ \left[ (\textcolor{black}{- \lambda \alpha_1}-  2g \alpha_1\alpha_3) + \left(\frac{\omega}{c}  \alpha_4  - 2g \alpha_1\alpha_5\right) {\cos \theta}  \right] \Sigma_y
+\left(-\frac{\omega}{c} \alpha_5  + 2 g \alpha_1 \alpha_4  \right){\sin \theta} \, \Sigma_z \right\} \vec{e}_y \nonumber\\
&=&  \left[ (\textcolor{black}{- \lambda \alpha_1}-  2g \alpha_1\alpha_3) + \left( - 2g \alpha_1\alpha_5\right) \right] \Sigma_y
 \vec{e}_y \nonumber\\
&=&  -\alpha_1 \left[ \lambda +  2g(\alpha_3+\alpha_5)\right] \Sigma_y  \vec{e}_y=0, \nonumber\\
\vec{{B}}
 &=& \left\{ \left[ (\lambda \alpha_2 + 2g \alpha_2 \alpha_3)+ \left( -k\alpha_4  + 2 g \alpha_2 \alpha_5 \right){\cos \theta} \right]\Sigma_y +\left( k \alpha_5 - 2g \alpha_2 \alpha_4 \right){\sin \theta}\, \Sigma_z \right\}\vec{e}_x \nonumber\\
 &=&  \left[ (\lambda \alpha_2 + 2g \alpha_2 \alpha_3)+ \left( 2 g \alpha_2 \alpha_5 \right) \right]\Sigma_y \vec{e}_x \nonumber\\
 &=&  \alpha_2 [\lambda + 2g (\alpha_3+\alpha_5)] \Sigma_y \vec{e}_x =0.
\end{eqnarray}
Hence, we would like to neglect this trivial case for both the fields $\vec{E}$ and $\vec{B}$ are zero. $\blacksquare$
\end{remark}

Next, we come to consider the nontrivial case with $k\neq 0$, $\omega\neq 0$. From Eq. (\ref{eq:analy-1}) and Eq. (\ref{eq:analy-2}), we can have the following 9 algebraic constraint equations:

\begin{subequations}
\begin{eqnarray}
&&  \alpha_1(\lambda + 2g\alpha_3)^2 + 2g\alpha_4\left(2g\alpha_1\alpha_4 - \frac{\omega}{c}\alpha_5\right)= 0, \label{eq:alg-1} \\
&&  (\lambda + 2g\alpha_3)\left(4g\alpha_1\alpha_5 - \frac{\omega}{c}\alpha_4\right)= 0, \label{eq:alg-2} \\
&&  4g^2 \alpha_1(\alpha_4^2 - \alpha_5^2)= 0, \label{eq:alg-3} \\
&&  2g\left[(\alpha_2^2 - \alpha_1^2)(\lambda + 2g\alpha_3) \right]= 0, \label{eq:alg-4} \\
&&  \alpha_5\left(k^2 - \frac{\omega^2}{c^2} - 4g^2(\alpha_1^2 - \alpha_2^2)\right) + 4g\alpha_4\left(\frac{\omega}{c}\alpha_1 - k\alpha_2\right)= 0, \label{eq:alg-5} \\
&& \alpha_4\left(k^2 - \frac{\omega^2}{c^2} - 4g^2(\alpha_1^2 - \alpha_2^2)\right) + 4g\alpha_5\left(\frac{\omega}{c}\alpha_1 - k\alpha_2\right) = 0, \label{eq:alg-6} \\
&&  \alpha_2(\lambda+2g\alpha_3)^2 + 2g\alpha_4(2g\alpha_2\alpha_4 - k\alpha_5) = 0, \label{eq:alg-7} \\
&&   (\lambda+2g\alpha_3)(4g\alpha_2\alpha_5 - k\alpha_4)= 0, \label{eq:alg-8} \\
&&  4g^2\alpha_2(\alpha_5^2-\alpha_4^2)= 0. \label{eq:alg-9} 
\end{eqnarray}
\end{subequations}

 After solving these 9 algebraic equations, we can have three families of exact solutions (generally $\lambda\neq 0$): (i) Linear waves, (ii) Nonlinear self-interacting waves, and (iii) Pure gauge solution.

%\subsubsection{Linear Wave}

\subsubsection{Linear Waves}

The parameters satisfy the following conditions
\begin{eqnarray}
\alpha_1 = 0,\qquad \alpha_2 = 0,\qquad \alpha_3 = -\frac{\lambda}{2g},\qquad \alpha_5 = 0,\qquad  \omega = k c,
\end{eqnarray}
where $\alpha_4$ is an arbitrary real constant, $\lambda$ is an arbitrary real constant (ensuring $\lambda y$ is dimensionless), $k$ is the wave number, $\omega$ is the frequency, and $g$ is the gauge coupling constant. The phase is defined as $\theta = kz - \omega t$. The gauge potentials are
\begin{eqnarray}
\varphi = 0,\qquad A_x=0,  \qquad A_z = 0,\qquad A_y = \alpha_3\,\Sigma_z + \alpha_4\sin\theta\;\Sigma_y,
\end{eqnarray}
and the corresponding electric and magnetic fields are

\begin{eqnarray}\label{eq:EB}
&&{\vec{E} = k\alpha_4\cos\theta\;\Sigma_y\;\vec{e}_y}, \nonumber\\
&& {\vec{B} = -k\alpha_4\cos\theta\;\Sigma_y\;\vec{e}_x}.
\end{eqnarray}
These fields satisfy the sourceless Yang--Mills equations and describe a linearly polarized plane wave propagating along the $z$-direction at the speed of light (due to the dispersion relation $\omega^2 = k^2 c^2$), with all nonlinear self-interactions vanishing identically.

\begin{remark}\textcolor{blue}{Why the first family of waves is called linear waves?} The reasons are

\begin{enumerate}
    \item \textbf{Nonlinear terms vanish:} $\varphi=0$, $A_x=A_z=0$, so $[\varphi,\vec{A}]=0$ and $\vec{A}\times\vec{A}=0$. Under such an
    \emph{Abelian limit}, the system reduces to Maxwell's equations with all the nonlinear commutators ${\rm i}g [ A_\mu, A_\nu]=0$.

    \item \textbf{Linear wave equations hold:} $\Box\vec{E}= \lambda^2 \vec{E}$, $\Box\vec{B}=\lambda^2 \vec{B}$, with $\Box=\frac{1}{c^2}\frac{\partial^2}{\partial t^2}-\vec{\nabla}^2$ and $\omega^2=k^2c^2$. When $\lambda=0$, one has $\Box\vec{E}= 0$ and $\Box\vec{B}=0$, which are the same as the electromagnetic waves for Maxwell's equations.

    \item \textbf{Superposition holds:} Linear combinations of solutions remain solutions.

    \item \textbf{Contrast with the second family (see below):} The second family has $\alpha_1,\alpha_2\neq0$, nonzero commutators, double frequency $2\omega$, and genuine self-interactions.
\end{enumerate}
Here, the \emph{Abelian limit} refers to the situation in a non-Abelian theory where, for a particular solution or under a certain limit, all nonlinear commutator terms effectively vanish, and the field equations reduce to those of Abelian (electromagnetic) theory. The first family of solutions is precisely the paradigm of this limit, which is why they are called ``linear waves''. Essentially, the first family embeds Abelian electromagnetic waves into the non-Abelian theory. Thus, the waves $\vec{E}$ and $\vec{B}$ in Eq. (\ref{eq:EB}) are Abelian  waves. $\blacksquare$
\end{remark}

\subsubsection{Nonlinear Self-Interacting Waves}

The parameters satisfy the following conditions:

\begin{eqnarray}
&&\alpha_1 = \alpha_2 = \frac{\eta k}{4 g }, \quad  \alpha_3 = \xi \alpha_4 - \frac{\lambda}{2g}, \quad \alpha_5 = \eta \alpha_4, \quad
\omega = k c, \quad
\nonumber\\
&&\eta = \pm 1,\quad \xi = \pm 1,\quad \alpha_4 \neq 0,\quad \lambda \in \mathbb{R},\quad \omega > 0.
\end{eqnarray}
where $\eta, \xi = \pm 1$ are discrete topological parity parameters, $\alpha_4$ is an arbitrary real constant (the wave amplitude), $\lambda$ is an arbitrary real constant (ensuring $\lambda y$ is dimensionless), $k$ is the wave number, $\omega$ is the frequency, and $g$ is the gauge coupling constant. The phase is defined as $\theta = kz - \omega t$. 
The algebraic basis is given by
\begin{eqnarray}
\Sigma_x = \cos(\lambda y)\,\sigma_x + \sin(\lambda y)\,\sigma_y,\qquad
\Sigma_y = -\sin(\lambda y)\,\sigma_x + \cos(\lambda y)\,\sigma_y,\qquad
\Sigma_z = \sigma_z.
\end{eqnarray}
The gauge potentials are
\begin{eqnarray}
\varphi = \alpha_1 \Sigma_x, \qquad A_x=0, \qquad
A_z = \alpha_2 \Sigma_x,\qquad
A_y = \bigl(\alpha_3 + \alpha_5\cos\theta\bigr)\Sigma_z + \alpha_4\sin\theta\;\Sigma_y,
\end{eqnarray}
The corresponding electric field $\vec{E} = E_y\,\vec{e}_y$ is
\begin{eqnarray}\label{eq:E-b}
E_y= \frac{k\alpha_4}{2}\left[(\cos\theta - \xi\eta)\,\Sigma_y - \eta\sin\theta\,\Sigma_z\right],
\end{eqnarray}
and the corresponding magnetic field $\vec{B} = B_x\,\vec{e}_x$ is
\begin{eqnarray}
B_x=-E_y=\frac{k\alpha_4}{2}\left[(\xi\eta - \cos\theta)\,\Sigma_y + \eta\sin\theta\,\Sigma_z\right].
\end{eqnarray}
These fields satisfy the sourceless Yang--Mills equations and describe a genuinely non-Abelian, self-interacting plane wave propagating along the $z$-direction at the speed of light (due to the dispersion relation $\omega = k c$). The parameter $\lambda$ remains free and appears only within the definitions of $\Sigma_x$ and $\Sigma_y$, while the constant terms involving $\lambda/(2g)$ in $\alpha_3$ cancel exactly with contributions from $-\nabla\varphi$ in the field calculations.

\begin{remark}
\textcolor{blue}{Why the second family of waves is called \textit{nonlinear self-interacting wave}?}
This solution is termed nonlinear self-interacting for the following reasons:

\begin{enumerate}
    \item \textbf{Non-vanishing commutator terms.}
    Unlike the linear waves (see \emph{ Remark~5}), here $\alpha_1 = \alpha_2 = \eta k/(4g) \neq 0$. Consequently $\phi = \alpha_1\Sigma_x \neq 0$ and $A_z = \alpha_2\Sigma_x \neq 0$, which make the commutators $[\phi,\vec{A}]$ and $\vec{A}\times\vec{A}$ non-zero. The nonlinear self-interactions in the Yang-Mills equations are genuinely active.

    \item \textbf{Constant offset term.}
    The electric and magnetic fields contain a $\theta$-independent piece proportional to $(\cos\theta - \eta\xi)$ (or $(\xi\eta - \cos\theta)$) that does not average to zero. Such a constant offset cannot arise in a linear (Abelian) wave; it originates from the balance between the gradient of $\varphi$ and the nonlinear commutator in the definition of $\vec{E}$.

    \item \textbf{Violation of superposition.}
    The system reduces to the algebraic constraints Eqs. (\ref{eq:alg-1})-(\ref{eq:alg-9}), which are quadratic in the amplitudes (e.g. $\alpha_1(\lambda+2g\alpha_3)^2$). A linear combination of two solutions with different $\alpha_4$ or different discrete parameters $\eta,\, \xi$ generally does not satisfy the YM equations. The wave is inherently non-linear.

    \item \textbf{Contrast with the linear wave family.}
    For the linear wave ($\alpha_1=\alpha_2=0$) all nonlinear terms vanish and the equations become Maxwell's equations. The wave, however, relies on the non-Abelian commutators to achieve an exact, light-speed propagating solution, thus it is a genuinely non-Abelian, self-interacting plane wave.
\end{enumerate}
In summary, the family of waves is called \textit{nonlinear self-interacting} because its very existence depends crucially on the nonlinear terms of the SU(2) Yang-Mills theory; it exhibits a constant offset, does not obey superposition, and its amplitude parameters are tied to the coupling $g$. The fields oscillate with the fundamental frequency $\omega$ (and wave number $k$) satisfying the usual dispersion relation $\omega = k c$. $\blacksquare$
\end{remark}

%\subsection*{Case 3: Wave Without Dispersion Constraint (Third family, general $\lambda$)}

\subsubsection{Pure Gauge Solution}

The parameters satisfy the following conditions:

\begin{eqnarray}
&& \alpha_1 = \eta\,\frac{\omega}{2gc},\qquad \alpha_2 = \eta\,\frac{k}{2g},\qquad \alpha_3 = -\frac{\lambda}{2g}, \quad \alpha_5 = \eta \alpha_4, \nonumber\\
&&\eta = \pm 1,\quad \alpha_4 \neq 0,\quad \alpha_1,\; \alpha_2 \neq 0,\quad \lambda \in \mathbb{R}.
\end{eqnarray}
where $\eta = \pm 1$ is a discrete topological parity parameter, $\alpha_4$ is an arbitrary real constant (the wave amplitude), $\lambda$ is an arbitrary real constant (ensuring $\lambda y$ is dimensionless), $k$ is the wave number, $\omega$ is the frequency, and $g$ is the gauge coupling constant.

Unlike the first two families, this solution imposes \textbf{no dispersion relation constraint} $\omega^2 = k^2 c^2$. The parameters $\omega$ and $k$ can be arbitrary real numbers (including $\omega = 0$, $k = 0$, or any nonzero values) and are completely independent.
The phase is defined as $\theta = kz - \omega t$.
The algebraic basis is given by
\begin{eqnarray}
\Sigma_x = \cos(\lambda y)\,\sigma_x + \sin(\lambda y)\,\sigma_y,\qquad
\Sigma_y = -\sin(\lambda y)\,\sigma_x + \cos(\lambda y)\,\sigma_y,\qquad
\Sigma_z = \sigma_z.
\end{eqnarray}
The gauge potentials are
\begin{eqnarray}
\varphi = \alpha_1 \Sigma_x,\qquad A_x=0, \qquad
A_z = \alpha_2 \Sigma_x,\qquad
A_y = \left(\alpha_3 + \alpha_5\cos\theta\right)\Sigma_z + \alpha_4\sin\theta\;\Sigma_y.
\end{eqnarray}

The corresponding electric field $\vec{E} = E_y\,\vec{e}_y$ is
\begin{eqnarray}
E_y &=& 0,
\end{eqnarray}
and the corresponding magnetic field $\vec{B} = B_x\,\vec{e}_x$ is
\begin{eqnarray}
B_x
&=& 0. 
\end{eqnarray}
These fields satisfy the sourceless Yang--Mills equations for arbitrary $\omega$ and $k$ without restriction like $\omega^2 = k^2 c^2$.

%\begin{acknowledgments}
%This work is supported by the Quantum Science and Technology-National Science and Technology Major Project (Grant No. 2024ZD0301000), and the National Natural Science Foundation of China (Grant No. 12275136).
%\end{acknowledgments}

%\appendix

\end{document}
